# Supplementary material for: Dynamic Time Warping for Lead-Lag Relationships in Lagged Multi-Factor Models
Source: arXiv:2309.08800 source file (2023-09-15)
Supplement: Supplementary file 1 [file supplementary.tex]

\setcounter{page}{1}
\begin{landscape}

\section{Supplemental material} \label{Supplemental}

\subsection{Equity data set: performance metrics for the entire grid -  rescaled to target volatility}
\label{equity_full_results}

Table \ref{tab: equity_grid} provides performance metrics for the entire grid (rescaled to target volatility). The experiment has
been set with the values $\alpha = 0.75$, $p = \{1,3,5,7\}$, $\delta = \{1,3,5,7\}$, and $K = \{5,10,15,20\}$.

\begin{small}
% [inline block 0: 1 envs, 87167 chars -> data_tex | \begin{longtable}{|p{2.5cm}p{1.2cm}p{0.1cm}p{0.1cm}p{0.5cm}p{0.5cm}{0.1cm}p{1.4cm}p{1.2cm}p{1.6cm}p{1.7cm}p{1cm}p{1cm}p{...]

\end{small}
\captionof{table}{Equity data set: performance metrics for the entire grid - rescaled to target volatility. The experiment has
been set with the values $\alpha = 0.75$, $p = \{1,3,5,7\}$, $\delta = \{1,3,5,7\}$, and $K = \{5,10,15,20\}$.}
\label{tab: equity_grid}

\subsection{ETF data set: performance metrics for the entire grid -  rescaled to target volatility}
\label{etf_full_results}

Table \ref{tab: etf_grid} provides performance metrics for the entire grid (rescaled to target volatility). The experiment has
been set with the values $\alpha = 0.75$, $p = \{1,3,5,7\}$, $\delta = \{1,3,5,7\}$, and $K = \{5,10,15,20\}$.

\begin{small}
% [inline block 1: 1 envs, 60543 chars -> data_tex | \begin{longtable}{|p{2.5cm}p{1.2cm}p{0.1cm}p{0.1cm}p{0.5cm}p{0.5cm}{0.1cm}p{1.4cm}p{1.2cm}p{1.6cm}p{1.7cm}p{1cm}p{1cm}p{...]

\end{small}
\captionof{table}{ETF data set: performance metrics for the entire grid - rescaled to target volatility. The experiment has
been set with the values $\alpha = 0.75$, $p = \{1,3,5,7\}$, $\delta = \{1,3,5,7\}$, and $K = \{5,10,15,20\}$.}
\label{tab: etf_grid}

\subsection{Futures data set: performance metrics for the entire grid -  rescaled to target volatility}
\label{futures_full_results}

Table \ref{tab: futures_grid} provides performance metrics for the entire grid (rescaled to target volatility). The experiment has
been set with the values $\alpha = 0.75$, $p = \{1,3,5,7\}$, $\delta = \{1,3,5,7\}$, and $K = \{5,10,15,20\}$.

\begin{small}
% [inline block 2: 1 envs, 87167 chars -> data_tex | \begin{longtable}{|p{2.5cm}p{1.2cm}p{0.1cm}p{0.1cm}p{0.5cm}p{0.5cm}{0.1cm}p{1.4cm}p{1.2cm}p{1.6cm}p{1.7cm}p{1cm}p{1cm}p{...]

\end{small}
\captionof{table}{Futures data set: performance metrics for the entire grid - rescaled to target volatility. The experiment has
been set with the values $\alpha = 0.75$, $p = \{1,3,5,7\}$, $\delta = \{1,3,5,7\}$, and $K = \{5,10,15,20\}$.}
\label{tab: futures_grid}

\end{landscape}
